# Supplementary material for: CCL4Rec: Contrast over Contrastive Learning for Micro-video Recommendation
Source: arXiv:2208.08024 source file (2022-08-17)
Supplement: Supplementary file 1 [file 6.Appendix.tex]

\section{Appendix}
\label{sec:appendix}
